# Supplementary material for: Learning Fast and Slow: PROPEDEUTICA for Real-time Malware Detection
Source: arXiv:1712.01145 source file (2021-10-17)
Supplement: Supplementary file 1 [file appendix.tex]

\subsection{Architecture of \textit{CNNLSTM} and \textit{LSTM} model}
\label{sec:app:twomodel}
Figure~\ref{fig:cnnlstm} and Figure~\ref{fig:lstm} depict the detailed architecture of \textit{CNNLSTM} and \textit{LSTM} model. We compare \deepm with these two models to show the improvement.
\begin{figure}[!htb]
	\centering
    \begin{subfigure}[b]{\linewidth}
    	\centering
        \includegraphics[width=\linewidth]{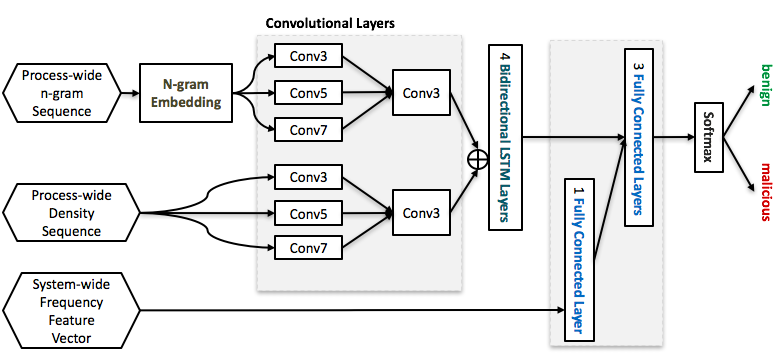}
        \caption{Illustration of \textit{CNNLSTM} model}
        \label{fig:cnnlstm}
    \end{subfigure}
    \begin{subfigure}[b]{\linewidth}
        \centering
      	\includegraphics[width=\linewidth]{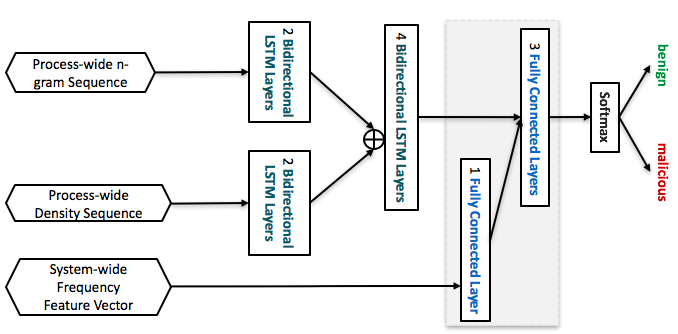}
      	\caption{Illustration of \textit{LSTM} model}
      	\label{fig:lstm}
    \end{subfigure}
    \caption{Architecture of \textit{CNNLSTM} and \textit{LSTM} model}
\end{figure}

\subsection{System Call Description}
\label{sec:app-syscall}
\begin{table*}[!htb]
\centering
\caption{The set contains 155 system calls, and is the \textbf{largest} set that have been hooked to our best knowledge.% The corresponding hex number can be found at \cite{ntapi}.
}
\scriptsize
\label{tab:syscall}
% \vspace{-5pt}
\begin{tabular}{|l|l|l|}
\hline
System Call Name & System Call Name &System Call Name\\ \hline\hline
oldNtCreateThread & oldNtCreateThreadEx & oldNtSetContextThread  \\ \hline
oldNtCreateProcess & oldNtCreateProcessEx & oldNtCreateUserProcess \\ \hline
oldNtQueueApcThread & oldNtSystemDebugControl & oldNtMapViewOfSection \\ \hline
oldNtOpenProcess & oldNtCreateProcess & oldNtCreateProcessEx  \\ \hline
oldNtOpenThread & oldNtQuerySystemInformation & oldNtSetInformationFile \\ \hline
oldNtQueryInformationFile & oldNtCreateMutant & oldNtDeviceIoControlFile \\ \hline
oldNtTerminateProcess & oldNtDelayExecution & oldNtQueryValueKey \\ \hline
oldNtQueryAttributesFile & oldNtResumeThread & oldNtCreateSection \\ \hline
oldNtLoadDriver & oldNtClose & oldNtOpenFile \\ \hline
oldNtNotifyChangeMultipleKeys & oldNtQueryMultipleValueKey & oldNtQueryObject \\ \hline
oldNtRenameKey & oldNtSetInformationKey & oldNtAllocateLocallyUniqueId \\ \hline
oldNtCreateDirectoryObject & oldNtCreateKey & oldNtCreateKeyTransacted \\ \hline
oldNtSetQuotaInformationFile & oldNtSetSecurityObject & oldNtSetValueKey \\ \hline
oldNtSetVolumeInformationFile & oldNtUnloadDriver & oldNtUnlockFile \\ \hline
oldNtUnmapViewOfSection & oldNtWaitForSingleObject & oldNtFlushInstructionCache  \\ \hline
oldNtQueryInformationProcess & oldNtSetInformationProcess & oldNtAlertThread \\ \hline
oldNtCallbackReturn & oldNtGetContextThread & oldNtAlertResumeThread \\ \hline
oldNtContinue & oldNtImpersonateThread & oldNtRegisterThreadTerminatePort \\ \hline
oldNtSuspendThread & oldNtTerminateThread & oldNtOpenMutant \\ \hline
oldNtQueryMutant & oldNtReleaseMutant & oldNtSetTimerResolution \\ \hline
oldNtSetSystemTime & oldNtQueryTimerResolution & oldNtQuerySystemTime \\ \hline
oldNtQueryPerformanceCounter & oldNtLockFile & oldNtOpenEvent \\ \hline
oldNtQueryInformationThread & oldNtQueryDirectoryFile & oldNtQueryEaFile \\ \hline
oldNtSetInformationThread & oldNtAccessCheckByTypeAndAuditAlarm & oldNtCreateEvent \\ \hline
oldNtCreateFile & oldNtDeleteFile & oldNtFlushVirtualMemory \\ \hline
oldNtFreeVirtualMemory & oldNtLockVirtualMemory & oldNtProtectVirtualMemory \\ \hline
oldNtUnlockVirtualMemory & oldNtReadVirtualMemory & oldNtWriteVirtualMemory \\ \hline
oldNtReadFile & oldNtWriteFile & oldNtWriteRequestData \\ \hline
oldNtCreatePort & oldNtImpersonateClientOfPort & oldNtListenPort \\ \hline
oldNtQueryInformationPort & oldNtRequestPort & oldNtAlpcAcceptConnectPort \\ \hline
oldNtAlpcConnectPort & oldNtAlpcCreatePort & oldNtAlpcCreatePortSection \\ \hline
oldNtAlpcDeleteResourceReserve & oldNtAlpcDisconnectPort & oldNtReplyWaitReceivePortEx \\ \hline
oldNtPrivilegeCheck & oldNtAlpcOpenSenderProcess & oldNtAlpcQueryInformation \\ \hline
oldNtAreMappedFilesTheSame & oldNtAssignProcessToJobObject & oldNtCancelSynchronousIoFile \\ \hline
oldNtCompressKey & oldNtCreateEventPair & oldNtCreateKeyedEvent \\ \hline
oldNtCreateProfile & oldNtCreateSemaphore & oldNtCreateSymbolicLinkObject \\ \hline
oldNtCreateTransactionManager & oldNtDebugContinue & oldNtDeletePrivateNamespace \\ \hline
oldNtDisableLastKnownGood & oldNtDisplayString & oldNtDrawText \\ \hline
oldNtEnumerateDriverEntries & oldNtEnumerateTransactionObject & oldNtGetCurrentProcessorNumber \\ \hline
oldNtGetNlsSectionPtr & oldNtGetPlugPlayEvent & oldNtGetWriteWatch \\ \hline
oldNtImpersonateAnonymousToken & oldNtInitiatePowerAction & oldNtIsProcessInJob \\ \hline
oldNtIsSystemResumeAutomatic & oldNtLoadKey & oldNtLoadKey2 \\ \hline
oldNtMakeTemporaryObject & oldNtMapUserPhysicalPagesScatter & oldNtModifyBootEntry \\ \hline
oldNtOpenPrivateNamespace & oldNtOpenResourceManager & oldNtOpenSemaphore \\ \hline
oldNtOpenSession & oldNtPrePrepareEnlistment & oldNtQueryInformationEnlistment \\ \hline
oldNtQueryInformationResourceManager & oldNtQueryInformationTransaction & oldNtQueryInformationWorkerFactory \\ \hline
oldNtReadOnlyEnlistment & oldNtRegisterProtocolAddressInformation & oldNtReplacePartitionUnit \\ \hline
oldNtResetWriteWatch & oldNtResumeProcess & oldNtSaveKeyEx \\ \hline
oldNtSetDefaultLocale & oldNtSetInformationDebugObject & oldNtSetInformationJobObject \\ \hline
oldNtSetInformationResourceManager & oldNtSetInformationTransactionManager & oldNtSetIntervalProfile \\ \hline
oldNtSetSystemPowerState & oldNtSetTimer & oldNtSinglePhaseReject \\ \hline
oldNtVdmControl & oldNtWaitLowEventPair &  \\ \hline

\end{tabular}
\end{table*}
